# Supplementary material for: Are We Ready to Embrace Generative AI for Software Q&A?
Source: arXiv:2307.09765 source file (2023-08-12)
Supplement: Supplementary file 1 [file 9_Supplementary.tex]

% Please add the following required packages to your document preamble:
% \usepackage{graphicx}
\begin{table*}[]
\begin{tabular}{l|p{15cm}} \toprule
Question Id   & 72166259    \\ \hline
Title         & Werkzeug server is shutting down in Django application   \\ \hline
Body          & \begin{tabular}[c]{@{}p{15cm}@{}}after updating the Werkzeug version from 2.0.3 to 2.1.0, I keep getting errors every time I run the server, and here is the error log: {[}LOG1{]} \\ this exception keep appearing while incrementing by 2 ( ('127.0.0.1', 44612) -\textgreater ('127.0.0.1', 44628) and the server crash\\ checking the changes log, I have found this detail: {[}LOG2{]}\\ here is the link to the changes log\\ it asks to check the documentation for alternatives but can not find any\\ please let me know how I would resolve this error, thank you NB: my python version is 3.8\end{tabular}   \\ \hline
\multirow{2}{*}{Human Answers} & \begin{tabular}[c]{@{}p{15cm}@{}}Literally just ran into this today. According to their (git repo issue 1715) and assuming you are running runserver\_plus, there are three options that worked for some users. The first worked for me:\\ 1. Not altering your files and adding the option --keep-meta-shutdown. My full command looks like python manage.py runserver\_plus --cert-file /path/to/cert.pem --key-file /path/to/key.pem --keep-meta-shutdown localhost:9000\\ 2. Comment out open lines 325 and 326 under your runserver\_plus.py\\ 3. \textbf
{Upgrading python to 3.10}\\ Hope this helps!\end{tabular}    \hline
& & \textbf{Evaluation}: \emph{This answer solves the question with the latest knowledge.} \\ \hline
\multirow{2}{*}{GPT Answers}  & \begin{tabular}[c]{@{}p{15cm}@{}}The error message suggests that the werkzeug.server.shutdown function has been removed in version 2.1.0 of Werkzeug, and that the code in your Django application is still trying to use it.\\ It is asking you to check the documentation for alternatives, but you are unable to find any.\\ One alternative to shutdown the server is to use os.\_exit(0) instead of werkzeug.server.shutdown function.\\ You can also use the CTRL+C to stop the server.\\ Additionally, you could also try \textbf{downgrading to version} 2.0.3 of Werkzeug if you are unable to find a suitable alternative.\\ \hline
\end{tabular} 
& & \textbf{Evaluation}: \emph{This answer solves the problem using common approach which is not specific to the problem.} \\
\end{tabular}%
\bottomrule
\caption{A Response for Overall Score Explanation}
\label{tab:my-table}
\end{table*}
